# Supplementary material for: Task-Driven Graph Attention for Hierarchical Relational Object Navigation
Source: arXiv:2306.13760 source file (2023-06-23)
Supplement: Supplementary file 1 [file 9-appendix.tex]

\appendix

\section{Appendix}
\label{s:appendix}

\subsection{Societal Impact}
This work presents HRON, a task that is a prerequisite for many long-horizon home-activities. Automation of such activities would facilitate the development of robotic home assistants, with potential benefits to several society groups, e.g., providing affordable care for the elderly, handicapped or sick. Such agents must safely navigate and localize objects required to attend to those under their care in large ecological scenes such homes, with dozens of possible objects and distractors, a challenge we address by introducing task-driven graph attention as part of their solution. However, such automation may carry negative secondary impacts that would need to be assessed appropriately by groups of social workers and economists. For example, such helpers may potentially displace human workers who could fulfill these caregiver roles in favor of cheaper automated alternatives. The pros of increased availability of home assistants must be weighed against the economic and societal impact of job displacement.

%%%%%%%%%%%%%%%%%%%%%%%%%%%%%%%%%%%%%%%%%%%%%%%%%%%%%%%%%%%%%%%%%%%%%
\subsection{Implementation Details}

\subsubsection{Policy Implementation and Neural Network Structure}
Our PPO implementation uses a custom feature extractor which combines the RGB-D, goal, and scene graph encodings into a common embedding. The goal embedding network consists of a 3-layer MLP (128, 128, 128), the RGB and depth encoders are 3-layer CNNs, and the graph encoder consists of a 3 heterogeneous graph transformer layers with ReLU activations followed by FC layers (128, 128, 128). The RGB, depth, and graph encoders produce vectors of length 256 which are concatenated to the embedded goal vector of length 128. This combined vector is feed through a 3-layer FC network (128, 128, 128) to provide the input to the value and action networks. We found that that it was important to have sufficient network depth after combining the features in order for the policy to leverage the graph features. The core PPO network consists of a dedicated value FC network (128, 128, 128) and policy FC network (128, 128, 128).

\subsubsection{Geodesic Reward}

A geodesic reward is used to densify the reward function for both directed and exploratory object navigation tasks. The geodesic reward is the difference between the previous and the current timestep's shortest traversable path to the target object. The reward is positive for approaching the target object, and negative for moving away. iGibson 2.0 provides the utility to compute the shortest path between any given two points by performing a shortest-path-length traversal across a traversability graph derived from a given scene's birds-eye traversable map.

\subsubsection{Computational Resources}
All experiments were run on an internal computer cluster. Each experiment required approximately 48 hours of training time on a node allocated 1 Nvidia GPU (3090 or Titan RTX), 60 gigabytes of RAM, and 20 CPU cores.

\subsubsection{Graph pooling}
The graph pooling mechanism can be expressed generically as the weighted mean of all node features after performing the graph convolution operations.
\begin{equation}\label{eqn:pool}
\mathbf{r} =  \sum_{i=1}^{N} \mathbf{w}_i\mathbf{x}_i.
\end{equation}

As seen in Eq. \ref{eqn:pool}, $w_i$ is $\frac{1}{N}$ for global mean pooling and the indicator variable $\text{\usefont{U}{bbold}{m}{n}1}_{x_i \in \text{task relevant}}$ for the task-driven graph attention. The indicator variable will take a value of 1 for task relevant nodes and 0 otherwise.
%%%%%%%%%%%%%%%%%%%%%%%%%%%%%%%%%%%%%%%%%%%%%%%%%%%%%%%%%%%%%%%%%%%%%

\subsection{Additional Experiments}

\subsubsection{Evaluating \ExperimentThree in Multiple Scenes}
We evaluate the robustness of our solution for \experimentthree by training and evaluating in eight different scenes from the iGibson 2.0~\cite{li2021igibson} dataset. These scenes model real homes with different layouts, numbers of rooms and objects. As seen in Fig.~\ref{fig:exploratory_nav_8_envs}, both the premapped and non-premapped version of our approach are able to successfully locate target objects. The final success rate is similar to the success rate observed for one scene, with longer training time due to the increased complexity.

\begin{figure}
\centering%
%\begin{subfigure}[b]{0.3\textwidth}
\begin{minipage}[t]{0.48\textwidth}%
\centering%
\includegraphics[width=\textwidth]{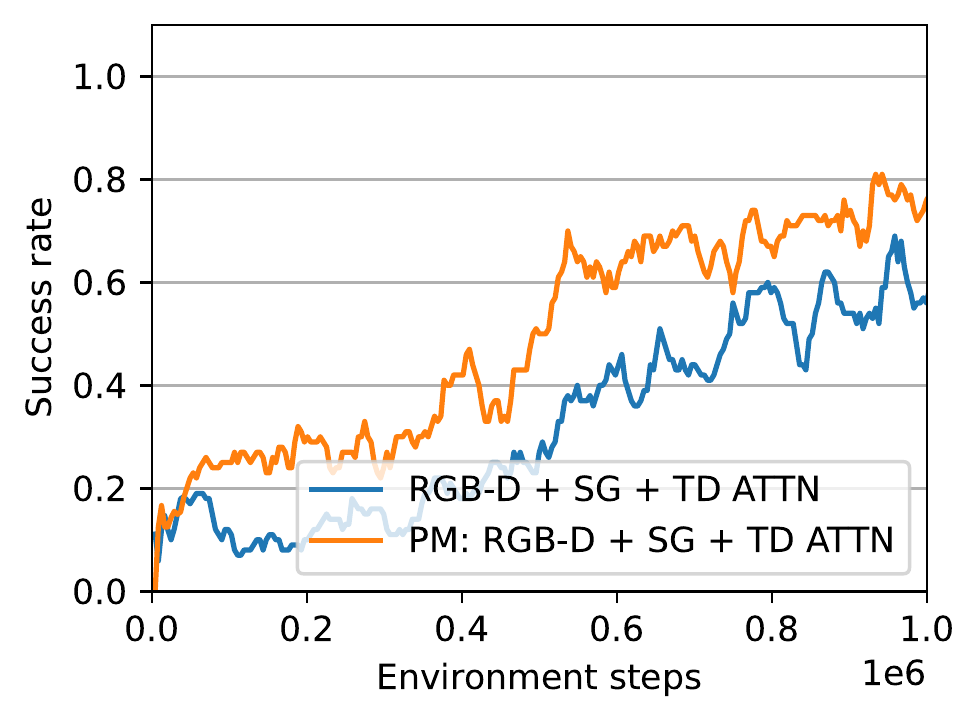}
\caption{Training results of the \experimentthree task in eight scenes. Both \sgattn and \sgattnpm are able to localize the target object when trained and evaluated in multiple scenes, showcasing the scalability of our approach.}%
\label{fig:exploratory_nav_8_envs}
%\end{subfigure}
\end{minipage}%
\hfill%
\begin{minipage}[t]{0.48\textwidth}%
%\begin{subfigure}[b]{0.3\textwidth}
\centering%
\includegraphics[width=\textwidth]{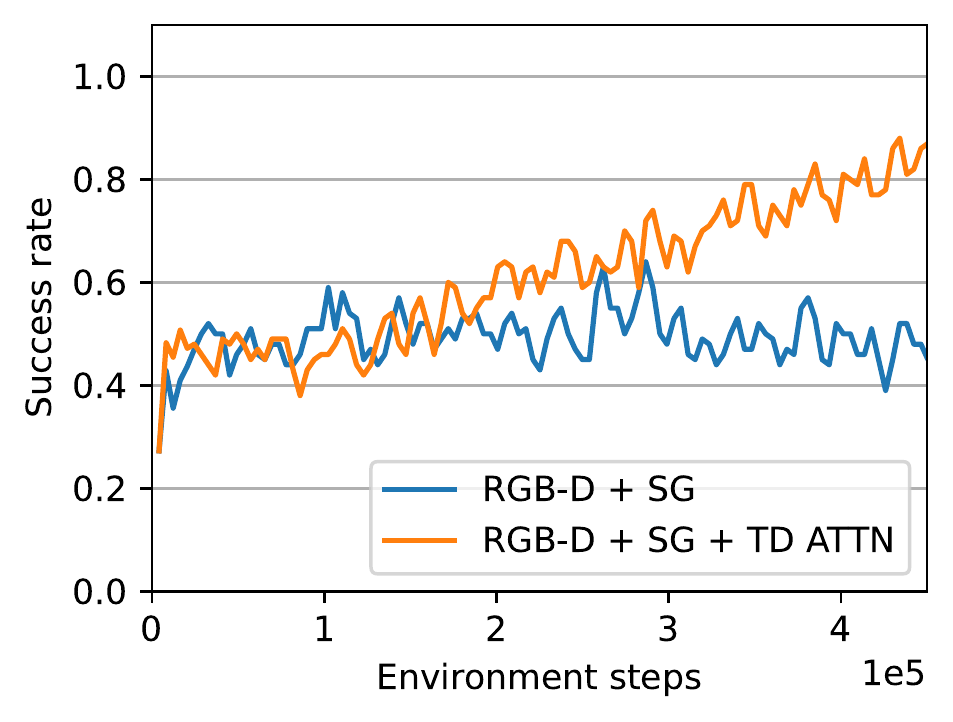}
\caption{Training results of \experimenttwo when introducing additional distractors. The presence of distractors lowers the performance of the \sgnoattn model. Introducing the task-driven attention mechanism (\sgattn) recovers the performance as evidenced by the improved success rate.}%
\label{fig:exp2_distractors}%
%\end{subfigure}%
\end{minipage}%
\end{figure}

\subsubsection{Impact of Distractors on \ExperimentTwo}
To further illustrate the impact of graph attention, we implemented a variant of \experimenttwo that includes distractor objects resembling that of \experimentone. As seen in Fig.~\ref{fig:exp2_distractors}, the presence of distractors cripples the performance of our model without attention (\textbf{\sgnoattn}) to chance-level. Introducing task-driven attention (\textbf{\sgattn}) mostly recovers the original performance.

\label{s:soc}

\subsubsection{Task-Driven vs. Learned Graph Attention}

Observing the evolution of the attention weights overtime (Fig.~\ref{fig:exp1_attn}), we see that the model learns to attend to the task-relevant objects as the task performance improves. The ability of the learned attention model to converge to the same performance as the task-driven attention is reflected in the data show in Fig.~\ref{fig:exp1_attn_results}, where we observe a longer training process to converge to the same performance.

\begin{figure}[h]
    \centering
    \includegraphics[width=0.15\textwidth]{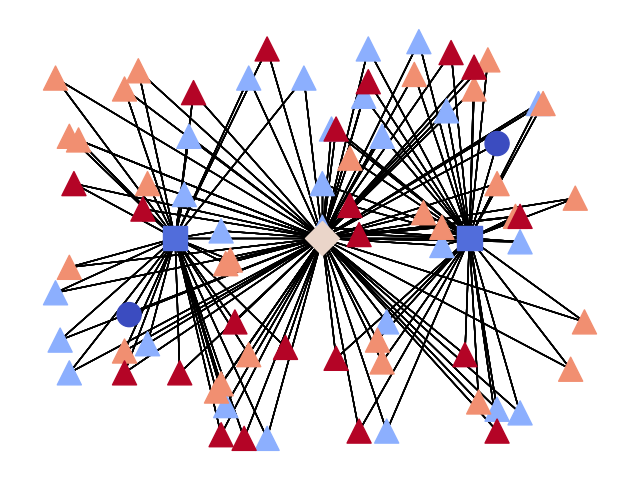}
    \includegraphics[width=0.15\textwidth]{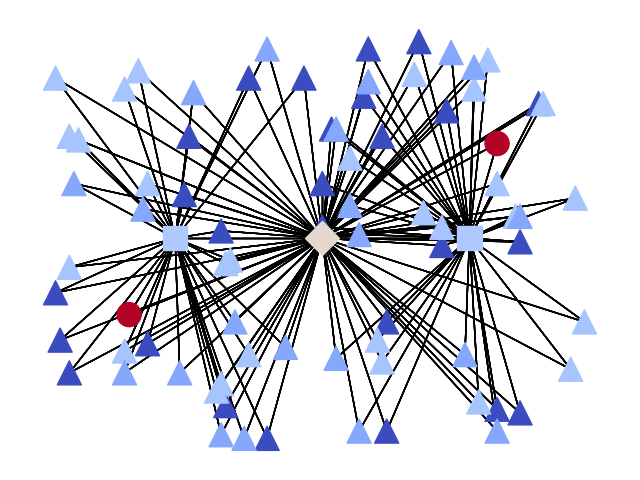}
    \includegraphics[width=0.15\textwidth]{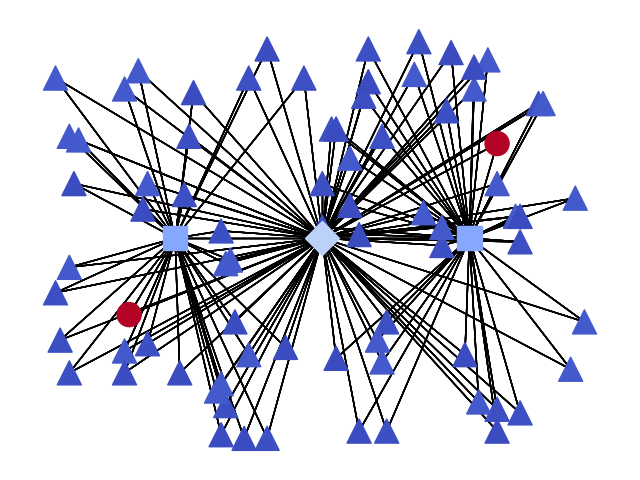}
    \caption{Evolution of learned attention over training in the \experimenttwo experiment with distractors. Resulting attention at the beginning of the training process (\textit{left}), at 5000 steps (\textit{middle}) and after convergence at 10000 steps (\textit{right}). For details on the experiment, we refer to Sec.~\ref{sec:experimental_setup}: the goal is to choose the right side as defined by the location of the circle with respect of the plane (squares in this figure). Highest attention is indicated with dark red and lowest attention is dark blue, with lighter red and blue indicating middle-high and middle-low attention. The attention shifts gradually towards task-relevant objects (circles and rectangles) and away from distractors (triangles). In comparison, our task-driven attention would focus on the two planes (squares) and the circles.}
    \label{fig:exp1_attn}
    %\vspace{128in}
\end{figure}

\label{s:soc}

\begin{figure*}
\centering
\includegraphics[width=0.32\textwidth]{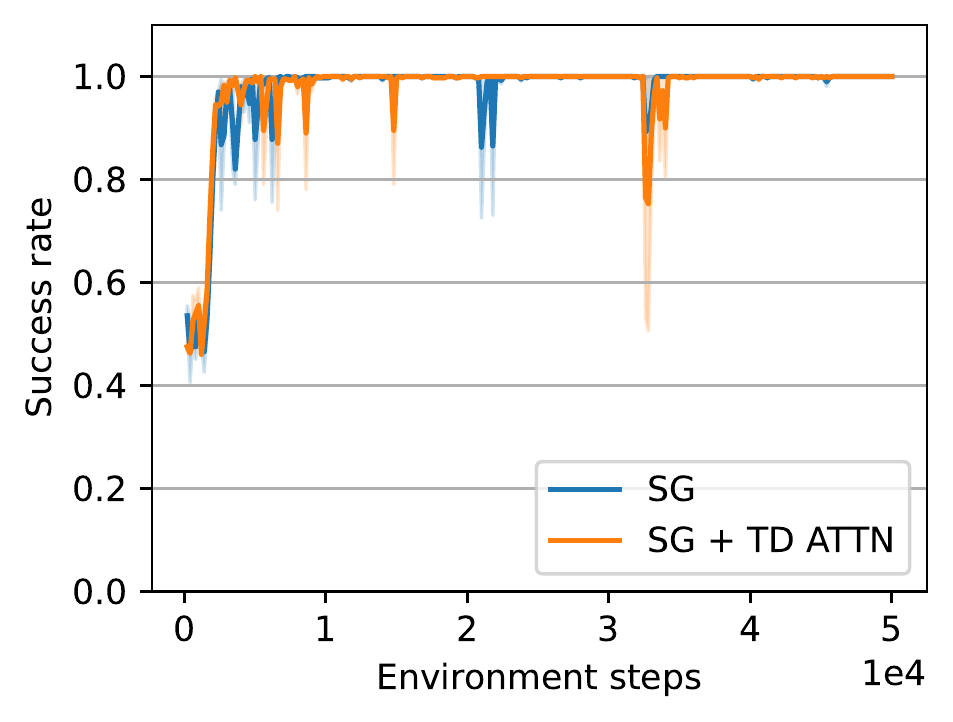}
\hfill
\includegraphics[width=0.32\textwidth]{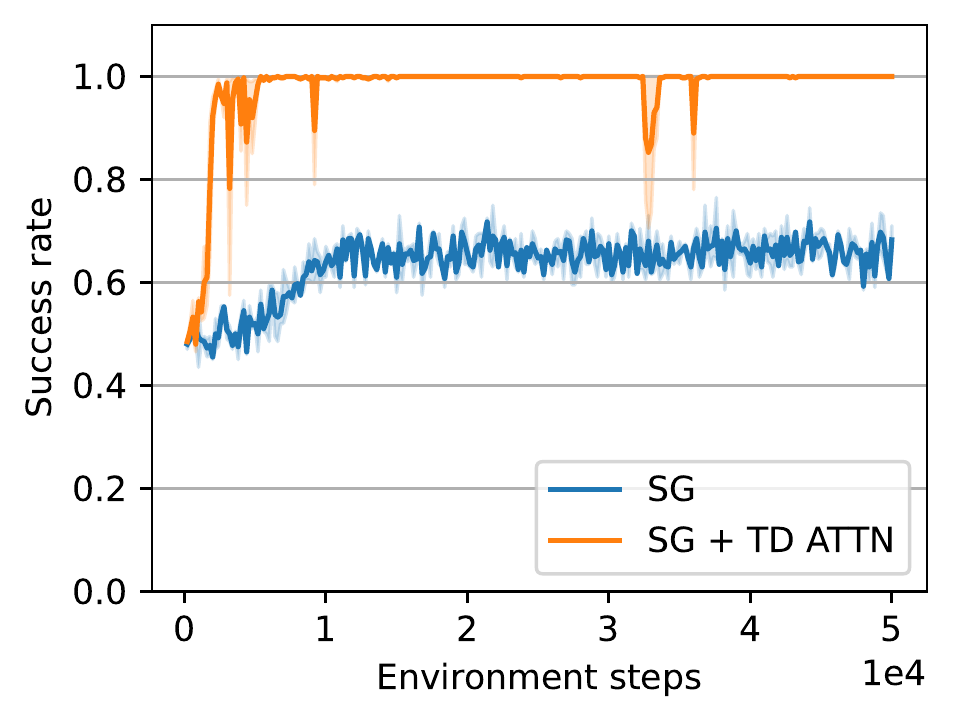}
\hfill
\includegraphics[width=0.32\textwidth]{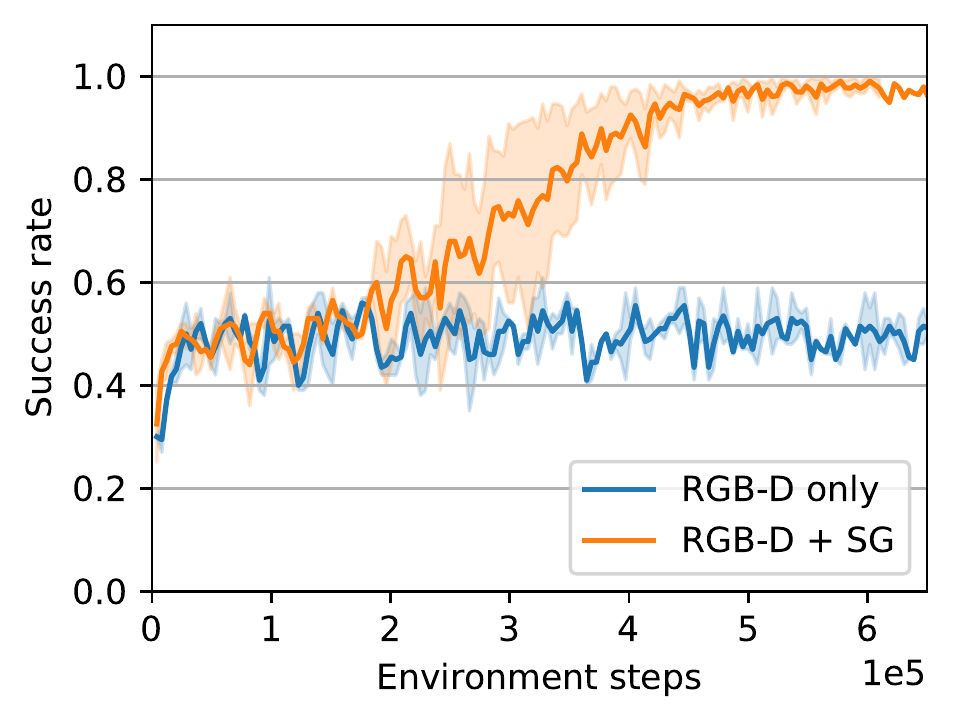}
\caption{Success Rate (SR) versus environment steps over training for the \experimentone\ and \experimenttwo\ tasks. The left two plots depict the \experimentone\ task with and without distractors, respectively. We observed that without attention, the performance of our model suffers significantly when there are many distractors. The rightmost plot depicts the \experimenttwo\ task. We observed that the \textbf{\sgnoattn} performs much better than \textbf{RGB-D only}, suggesting that scene graphs are effective representation for tasks that require relational reasoning.}
\label{fig:exp1_exp2}
\end{figure*}

\begin{figure}[h]
\begin{center}
    \includegraphics[width=0.4\textwidth]{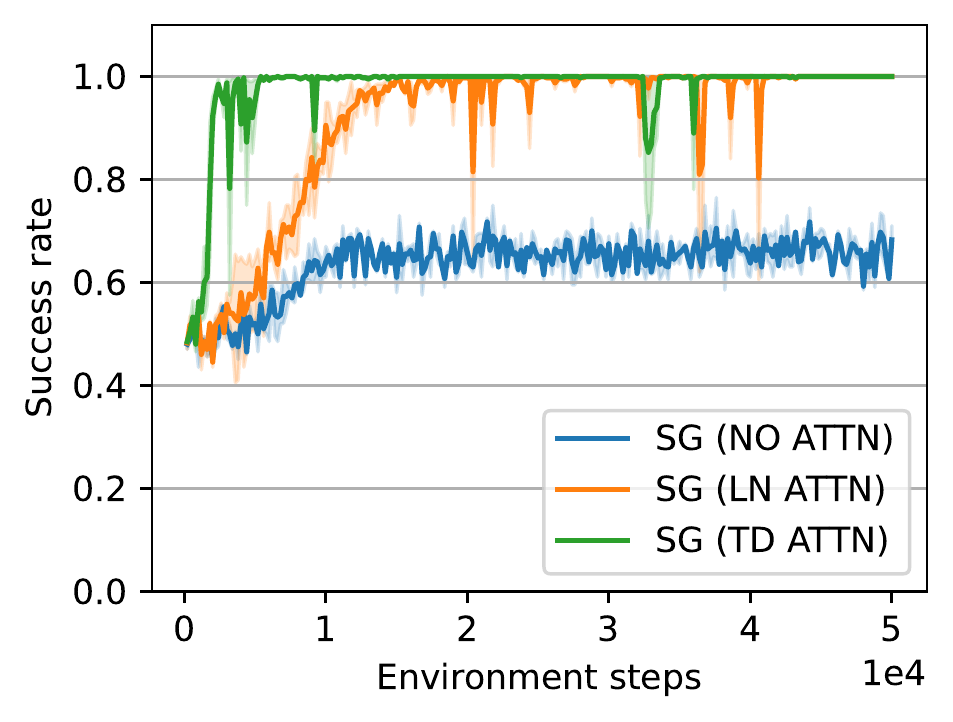}
    \caption{Comparison of task-driven and learned attention in the \experimentone experiment with distractors: Compared to no attention (\textit{blue}), learned attention (\textit{orange}) recovers the performance of the task-driven attention (\textit{green}) but requires more training steps due to the additional learning problem of co-training the attention layer.}
    \label{fig:exp1_attn_results}
\end{center}
\end{figure}

\begin{figure*}
    \centering
    \includegraphics[height=0.2\textwidth]{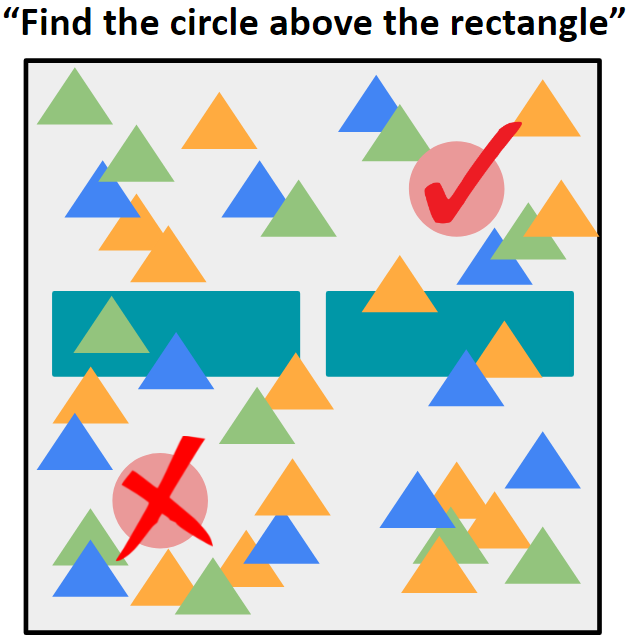}
    \includegraphics[height=0.2\textwidth]{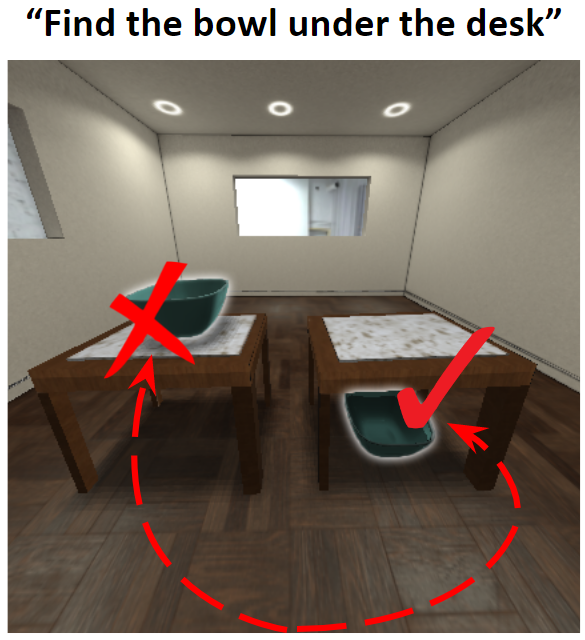}
    \includegraphics[height=0.2\textwidth]{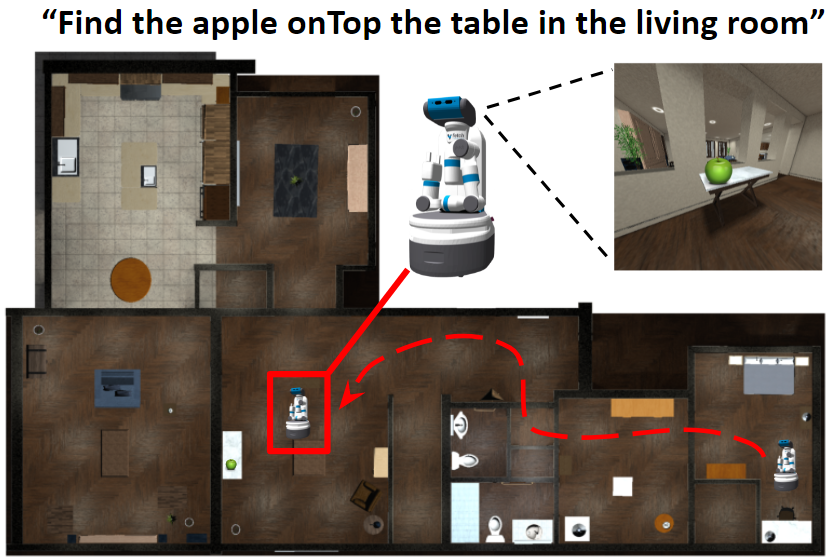}
    \caption{Three concrete tasks that illustrate relational object reasoning: \experimentone, \experimenttwo, and \experimentthree. In \experimentone~(left), given a relational object goal such as ``the circle above the rectangle'', the agent should output a binary choice (\texttt{left}/\texttt{right}) that corresponds to the side of the environment that satisfies the goal. In \experimenttwo and \experimentthree~(middle, right), given a relational object goal such as ``the apple on top of the table in the living room'', the agent should output a sequence of discrete navigation actions (\texttt{forward}/\texttt{backwards}/\texttt{left}/\texttt{right}/\texttt{stop}) to find and get close enough to the target object.}
    \label{fig:problem_setup}
\end{figure*}
